# Supplementary material for: Attosecond nanoplasmonic streaking of localized fields near metal nanospheres
Source: arXiv:1105.2738 ancillary file (2011-09-15)
Supplement: Supplementary file 1 [file Suessmann2011_Supp_inf.pdf]

# Attosecond nanoplasmonic streaking of localized fields near metal nanospheres - Supplementary Information

Frederik Süßmann and Matthias F. Kling

Max-Planck-Institut für Quantenoptik, Hans-Kopfermann-Straße 1, D-85748 Garching, Germany

## PLASMONIC PROPERTIES OF AU NANOPARTICLES

The plasmonic response of the Au nanospheres was calculated using Mie theory and is dependent on the driving wavelength, the nanoparticle size, material, composition, and its surrounding. For computing the electric field distributions the SPLaC package was used [1]. The optical properties of Au in the visible are modeled by

$$\epsilon(\lambda) = \epsilon_{\infty} \left( 1 - \frac{1}{\lambda_p^2 \left( \frac{1}{\lambda^2} + \frac{i}{\mu_p \lambda} \right)} \right) + \sum_n \frac{A_1}{\lambda_n} \left[ \frac{e^{i\psi}}{\frac{1}{\lambda_n} - \frac{1}{\lambda} - \frac{i}{\mu_n}} + \frac{e^{-i\psi}}{\frac{1}{\lambda_n} + \frac{1}{\lambda} + \frac{i}{\mu_n}} \right] \quad (1)$$

A fit to the experimental data reported by Palik [2] yielded  $\epsilon_{\infty} = 1.54$ ,  $\lambda_p = 177.5$  nm,  $\mu_p = 14500.0$  nm,  $A_1 = 1.27$ ,  $\lambda_1 = 470.0$  nm,  $\mu_1 = 1900.0$  nm,  $A_2 = 1.1$ ,  $\lambda_2 = 325.0$  nm,  $\mu_2 = 1060.0$  nm,  $\psi = -\pi/4$  [1]. As the experiment takes place in vacuum, the dielectric constant of the surrounding was set to  $\epsilon_s = 1$ . Fig. 1a) shows the wavelength dependent resonance curve for the near-field enhancement  $\sigma = E_p/E_0$  and Fig. 1b) the wavelength dependent phase shift  $\Delta\phi_p$  of the plasmonic field with respect to the driving laser field for different Au sphere diameters. For diameters smaller than 100 nm, only a small increase in field enhancement with increasing sphere size can be discerned. With increasing diameter beyond 100 nm a significant red shift and broadening of the resonance spectrum occurs. Particles with 200 nm diameter are resonant with the driving wavelength, but do not show much higher enhancement than smaller particles.

## INITIAL CONDITIONS FOR COMPLETE SPECTROGRAMS

In order to generate streaking spectrograms, that are expected from the experiment, a large number of electron trajectories were integrated. The initial conditions were randomized with probabilities accounting for the experimental conditions.

The emission position was randomized on the half sphere facing the detector, as electrons from the other side are unlikely to reach the detector. If the particles are assumed to be opaque for the XUV photons, emission of such photons would be limited to the half sphere

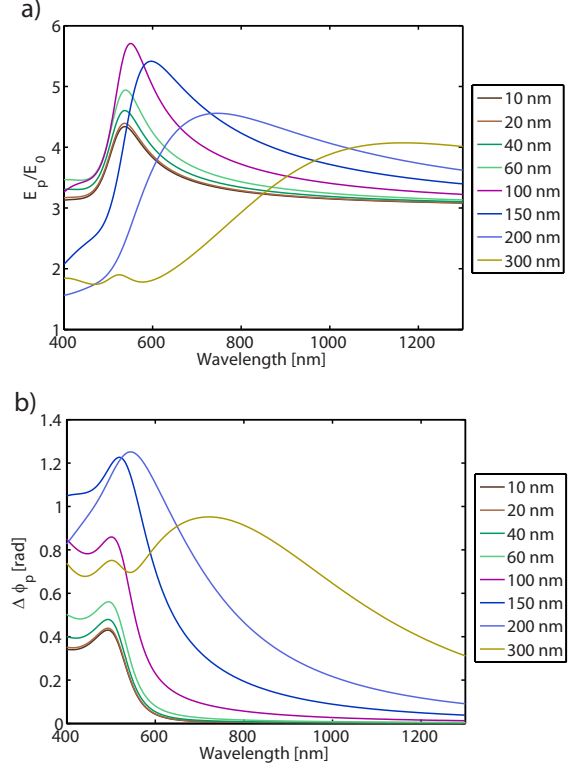

FIG. 1: Wavelength dependent plasmonic field enhancement (a) and phase shift of the plasmonic field with respect to the driving field (b) for different Au nanospheres with indicated diameters as calculated by Mie theory.

that is illuminated by the XUV. As the particles under consideration have diameters between 10–100 nm, transmission of the XUV photons can reach values close to unity. Therefore emission can also take place at the back side of the sphere. To obtain the correct emission probability especially for small spheres, transmission of XUV through the nanosphere and emission from the back side was included in the calculations. The relation between XUV intensities at the front and backside at a position given by the spherical coordinates  $\varphi$  and  $\theta$  is

$$A_b(\varphi, \theta) = A_f(\varphi, \theta) \exp(-\mu_a n \sin(\varphi) \sin(\theta) d). \quad (2)$$

Here  $d$  is the sphere diameter,  $\mu_a$  the atomic photoabsorption cross section and  $n$  is the atomic density of the solid [3]. From eq. 2 an effective probability for emission from a randomized position  $(\varphi, \theta)$  can be derived. This probability influences the relative statistical weight be-

tween contributions with small and large  $\alpha$ . The effect is largest for medium sized spheres ( $d = 20 - 40$  nm), while it is almost negligible for smaller and larger spheres. Emission of electrons was assumed to be isotropic, so the launch angle of an emitted electron was randomized within the acceptance angle of the detector ( $\pm 22^\circ$  to the x-axis). The initial kinetic energy was assumed to be Gaussian distributed (FWHM 5 eV) around the center photon energy subtracted by the work function. Similarly, the emission time was Gaussian distributed around a fixed delay value accounting for the XUV pulse length of 200 as.

### NANOPLASMONIC FIELD RECONSTRUCTION FROM $\alpha=0^\circ$ CONTRIBUTION

Generally, due to the complex contribution of various electron trajectories to the obtained attosecond nanoplasmonic streaking spectra, the spatio-temporal properties of the nanoplasmonic field can only be reconstructed by numerical simulations (similar to the ones shown in the main text, which have to be compared to recorded spectra). For well-chosen parameters, however, certain approximations might allow an analytic reconstruction of the nanoplasmonic field at the nanoparticle surface. The procedure is outlined below.

The equation of motion

$$\vec{v}_f(t_e) = \vec{v}_0 - \int_{t_e}^{\infty} dt \frac{\vec{E}(\vec{r}, t)e}{m}. \quad (3)$$

is in this form not integrable. But for the high XUV photon energy of 105 eV and NIR intensities of  $10^{12}$  W/cm<sup>2</sup> used here, an electron is accelerated by less than 10 percent with respect to its initial velocity  $v_0$  by the plasmonic field. The electron's distance to the surface of the sphere (with radius  $R = d/2$ ) at time  $t$  can therefore be approximated by  $r(t) \approx R + v_0(t - t_e)$ , where  $t_e$  is the emission time of the electron. The spatial decay of the field along the polarization axis is well described within the dipole approximation for the particle sizes considered here, resulting in  $E(r, t) \sim E(R, t)R^3/r(t)^3$ . In order to facilitate an integration of the electrons equation of motion in this field, the spatio-temporal decay of the field is expanded into a sum of exponentials

$$\begin{aligned} E(r, t) &= E(R, t) \times \sum_n a_n \exp(-(r(t) - R)/\varrho_n) \\ &\approx E(R, t) \times \sum_n a_n \exp(-(t - t_e)/\zeta_n), \end{aligned} \quad (4)$$

with  $\zeta_n = \varrho_n/v_0$  and  $\varrho_n$  being the decay constants. The temporal profile of the plasmonic near-field for small diameter particles (of 10 nm and 100 nm used here), which are off-resonant to the driving laser frequency, is

assumed to follow a Gaussian profile similar to the driving laser pulse:

$$E(R, t) = E_p \exp\left(\frac{-t^2}{\tau^2}\right) \cos(\omega t + \phi), \quad (5)$$

where  $E_p$  is the peak electric field amplitude at the sphere surface. Under this assumption the electric field (which accelerates and decelerates XUV-emitted electrons) is a function of time only given by eq 5 and 4. Integrating the equation of motion for an emitted electron gives the final velocity as a function of the emission time  $t_e$  for the  $\alpha = 0^\circ$  ( $n = 1$ ) contribution:

$$\begin{aligned} v_f(t_e) &= v_0 + E_p \tau R e \left[ \text{Erfc}\left(\frac{t_e}{\tau} + \frac{\tau - i\tau\zeta\omega}{2\zeta}\right) \right. \\ &\quad \left. \times \exp\left(i\phi + \frac{t_e}{\zeta} - \frac{\tau^2(i + \zeta\omega)^2}{4\tau^2}\right) \right], \end{aligned} \quad (6)$$

$\tau$ ,  $\phi$  and  $\omega$  are the pulse length, carrier envelope phase and angular frequency of the near field. The initial velocity  $v_0$  is fixed corresponding to a kinetic energy of 100 eV. When applying the fit, a complete reconstruction of all fit parameters is not unique, such that a complete reconstruction both in space and time is ambiguous. The temporal evolution of the near-field at the surface, however, can be reconstructed via fixing values for  $\zeta_n$  by fitting the spatial decay given by eq. 4 to the dipole approximation. For sufficiently large spheres (e.g. for 100 nm spheres) the  $\alpha = 0^\circ$  contribution can be obtained directly from the streaking spectrogram (for the streaking spectrogram see Fig. 4 in the main text). Figure 2a) shows the reconstructed streaking waveform (red) compared to the directly simulated one (blue). The simulated and reconstructed field evolution acting on an electron emitted at  $t = t_e = 0$  is shown in b). The agreement is very reasonable. The reconstructed field evolution on the sphere's surface at  $\alpha = 0^\circ$  shown in c) is similarly accurate and all pulse parameters are obtained with a maximal error of 5%. The analysis presented here can be extended to more generic field waveforms by modifying eq. 5 to assume a different time dependence of the near-field.

### COUNT RATE APPROXIMATION

In order to test the possibility to implement the suggested attosecond nanoplasmonic streaking on isolated nanospheres experimentally, the count rate for XUV-emitted electrons was estimated as detailed below. Direct (un-scattered) electrons are assumed to be emitted from a thin surface volume within a depth  $h = 0.5$  nm, as the mean free path of an electron with a kinetic energy of 100 eV is about 0.5 nm [4]. The total number of these electrons emitted per XUV pulse and surface area

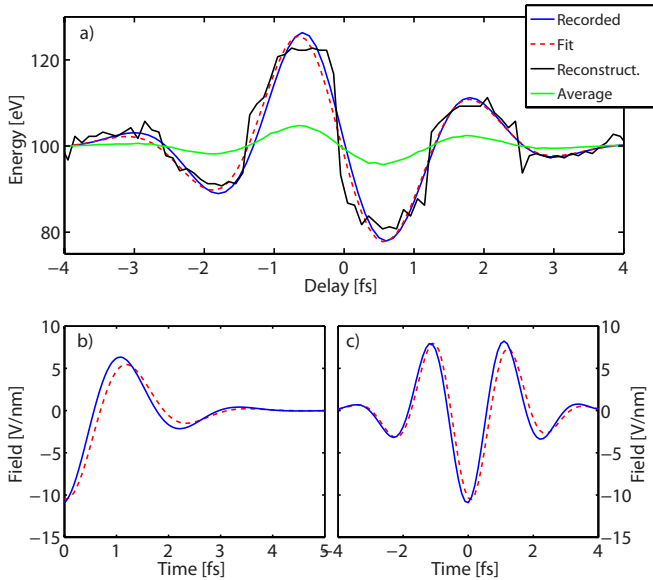

FIG. 2: a) Retrieval (black) and fit (red) of the  $\alpha = 0^\circ$  contribution to the streaking spectrogram for 100 nm Au spheres. For comparison the true  $\alpha = 0^\circ$  streaking waveform is shown in blue. b) Acceleration field of an electron liberated at time  $t = t_e = 0$  from simulation (blue) and fit (red). c) Reconstructed near-field (red) for a) as compared to the field evolution entering the simulation (blue).

is proportional to the photoabsorption cross section  $\sigma_a$ :

$$c_e = \rho h \sigma_a I_{ph}, \quad (7)$$

where  $\rho = 58.4 \text{ nm}^{-3}$  is the atomic density of the solid and  $I_{ph} = N_{ph} r_f^{-2}$  is the number of photons per laser shot per area incident on the sample.  $\sigma_a$  is assumed to be  $10.9 \times 10^{-18} \text{ cm}^2$  [3]. Multiplying eq. 7 with the area of the nanosphere  $A = R^2 \pi$  facing the time-of-flight (TOF) detector (as only these electrons can reach the detector) gives the average count rate  $n_e$  per particle

$$n_e = c_e \pi R^2 p_d, \quad (8)$$

with  $p_d$  being the probability for an emitted electron to reach the TOF-detector. Electrons are assumed to be emitted isotropically. The acceptance angle of the TOF detector taken from a commercially available TOF spectrometer [5] as  $\pm 22^\circ$ , resulting in a probability of  $p_d \approx 1\%$  for an emitted electron to be detected. Typical values for a table-top XUV source are  $10^5$  photons per laser shot and a focal spot size of  $r_f = 10 \mu\text{m}$  [6]. For a particle radius of 50 nm, this gives approximately  $3 \times 10^{-3}$  counts per particle and laser shot. The expected overall count rate is given by

$$j = V_i n_e f \rho_p, \quad (9)$$

where ( $V_i = \pi r_f^2 l$ ) is the laser - nanoparticle interaction volume,  $f$  the laser repetition rate and  $\rho_p$  the number

density of nanoparticles. The extent of the interaction volume in laser propagation direction is assumed to be  $l = 500 \mu\text{m}$ . The number density of nanoparticles can be expressed as a function of the parameters most relevant to an experimental realization

$$\rho_p = 2 \times 10^6 N_{ph}^{-1} R^{-2} f^{-1} j \text{ m}^{-3}. \quad (10)$$

Current table-top XUV sources operate at repetition rates in the kilohertz regime [7], while at the same time overall acquisition times are limited by the laser stability (in particular also the time the carrier-envelope phase of the laser can be actively stabilized). In order to perform measurements with sufficient statistics within a reasonable short overall time a count rate of at least 100 counts/s would be desirable. Assuming a repetition rate of 10 kHz and a photon number of  $10^5$  per laser shot provided by a table-top XUV source, a dense nanoparticle cloud with densities  $\rho_p$  exceeding  $1 \times 10^8 \text{ cm}^{-3}$  has to be utilized to reach the desired count rate. Such dense targets can be realized by laser ablation [8]. Alternatively, the number of XUV photons incident on the particle can be increased if the particles are produced by e.g. aerosol techniques and trapped at the focus of the XUV pulse (see e.g. [9] for a suitable approach)). While both approaches are challenging, employing an XUV light source with high flux such as the one expected to emerge at the European Light Infrastructure (ELI) [10], would facilitate a sufficient count rate in conjunction with a standard aerosol particle source delivering particle densities of ca.  $1 \times 10^6 \text{ cm}^{-3}$ : for an envisioned flux of e.g.  $10^{12}$  photons/s, a count rate of 1000 counts/s could be reached, facilitating a straightforward experimental implementation.

- 
- [1] E. C. L. Ru and P. G. Etchegoin, *Principles of Surface-Enhanced Raman Spectroscopy and Related Plasmonic Effects* (Elsevier, 2009).
  - [2] E. D. Palik, *Handbook of optical constants of solids III* (Academic Press, 1998).
  - [3] B. Henke, E. Gullikson, and J. Davis, *At. Data Nucl. Data Tab.* **54**, 181 (1993).
  - [4] S. Tanuma et al., *Surf. Interface Anal.* **17**, 911 (1991).
  - [5] S. Käs Dorf, *Geräte für forschung und industrie*, URL [www.kaesdorf.de](http://www.kaesdorf.de).
  - [6] M. Schultze et al., *New J. Phys.* **9**, (2007).
  - [7] F. Krausz and M. Ivanov, *Rev. Mod. Phys.* **81**, 163 (2009).
  - [8] S. Noel et al., *Appl. Surf. Sci.* **253**, 6310 (2007).
  - [9] J. Meinen et al., *Rev. Sci. Instr.* **81**, 085107 (2010).
  - [10] J.-P. Chambaret et al., *Proc. SPIE* **7721**, 1D (2010).
